# Supplementary material for: Transition from quasi-unidirectional to unidirectional guided resonances in leaky-mode photonic lattices
Source: arXiv:2312.00283 source file (2023-12-01)
Supplement: Supplementary file 1 [file Supplementary-Information.pdf]

# Supplementary Information for

## Transition from quasi-unidirectional to unidirectional guided resonances in leaky-mode photonic lattices

### 1. The relationship between $h_u$ , $h_d$ , and $w$

In the main text, we demonstrated that quasi-UUGRs and quasi-DUGRs progressively evolve into genuine UUGRs and DUGRs, respectively, as the grating thickness  $h$  is varied, while maintaining a fixed grating width of  $w = 0.4 \Lambda$ . Through extensive FEM simulations, we have verified that UUGRs and DUGRs can also be identified by tracking the evolutions of quasi-UUGRs and quasi-DUGRs with variations in  $h$  for different  $w$  values. Figure S1 presents the normalized grating thicknesses  $h_u$  and  $h_d$ , at which UUGRs and DUGRs are observed, as a function of the grating width  $w$ . For the fixed values of  $w$  (or  $h$ ), both the UUGRs and DUGRs can be achieved by tuning  $h$  (or  $w$ ) values gradually. The significance of ZCG-based unidirectional light emitters lies in their ease of fabrication using existing nanofabrication technologies, making them highly relevant for practical applications.

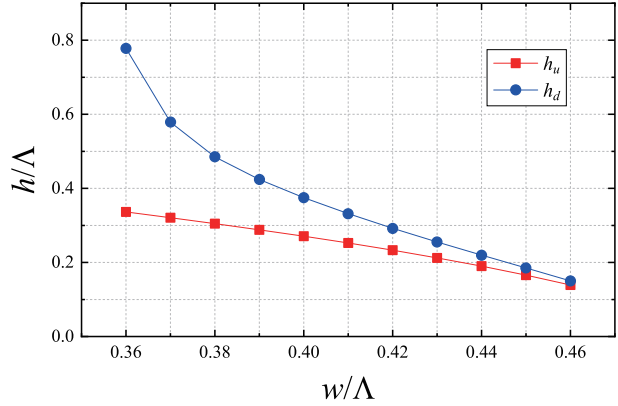

FIG. S1.  $h_u$  and  $h_d$  as a function of  $w$ .

### 2. Topological nature of UGRs induced by interband coupling in ZCGs

According to the topological charge framework, topologically enabled UGRs emerge at specific  $k$  points, where a pair of  $C$  points carrying half-integer topological charges merge [S1, S2]. We herein confirm that the topological charge framework in 2D momentum space is valid for elucidating the creation of interband-coupling-induced UGRs in ZCGs.

**Polarization vector fields and  $C$  points** In leaky-mode photonic lattices, above the light line and below the diffraction limit, an eigenmode with an in-plane wave vector  $\mathbf{k}_{||}$  couples to a propagating plane wave with the same  $\mathbf{k}_{||}$ . To investigate the dynamics of polarization singularities, including  $C$  points, BICs, and quasi-UGRs, it is crucial to calculate the polarization vectors of the far-field radiation projected on to  $x$ - $y$  plane given by  $\mathbf{c}(\mathbf{k}_{||}) = c_x(\mathbf{k}_{||})\hat{x} + c_y(\mathbf{k}_{||})\hat{y}$ . When plotting polarization vectors in  $k_x$ - $k_y$  space, polarization singularities carry topological charges, which are defined as [S3–S5]:

$$q = \frac{1}{2\pi} \oint_L d\mathbf{k}_{||} \cdot \nabla_{\mathbf{k}_{||}} \phi(\mathbf{k}_{||}), \quad (\text{S.1})$$

where  $L$  is a closed path encircling the polarization singularity in the counterclockwise direction, and  $\phi(\mathbf{k}_{||}) = \frac{1}{2}\arg[S_1(\mathbf{k}_{||}) + iS_2(\mathbf{k}_{||})]$  is the angle between its long axis of the polarization ellipse and the  $x$  axis, and  $S_i(\mathbf{k}_{||})$  represents the Stokes parameter of  $\mathbf{c}(\mathbf{k}_{||})$ . At  $k$  points where the polarization vector cannot be defined in a continuous manner, polarization singularities with nonzero topological charges are manifested. BICs and UGRs appear at  $k$  points where  $S_1 = S_2 = S_3 = 0$ . In contrast,  $C$  points emerge under the condition  $S_1 = S_2 = 0$  and  $S_3 = \pm 1$ . The topological charge  $q$  quantifies the winding of the polarization vector around a closed loop  $L$ . When  $L$  encloses BICs or UGRs, the topological charge  $q$  takes integer values. If  $L$  encloses  $C$  points,  $q$  takes half-integer values.

**Generation of UGRs by merging paired  $C$  points** In the main text, we confirmed that interband-coupling-induced UUGRs and DUGRs are observed at grating thicknesses  $h/\Lambda = h_u = 0.2708$  and  $h/\Lambda = h_d = 0.375$ , respectively, with fixed values of  $w/\Lambda = 0.4$  and  $t/\Lambda = 0.5$ . Herein, we first demonstrate that the interband-coupling-induced UUGR when  $h/\Lambda = h_u = 0.2708$  is generated at the merging point of paired topological charges with  $q = +1/2$ . The verification for the DUGR at  $h/\Lambda = h_d = 0.375$  is presented subsequently. Figure S2(a) illustrates the polarization vector fields of downward radiation corresponding to a grating thickness of  $h/\Lambda = h_u = 0.2708$ . Here, the polarization vectors are visualized as streamlines that trace the major axis of the polarization ellipses. It is evident from Figure S2(a) that the polarization vectors encircle the UUGR situated at  $(k_x, k_y)/K = (0.214731, 0)$ , indicating that the UUGR is endowed with a topological charge of  $q = +1$ . Far-field polarization states, as illustrated in Fig. S2(b), shows that there is no circularly polarized  $C$  point observed when  $h/\Lambda = h_u$ . To ascertain whether a UUGR is generated at the convergence point of paired  $C$  points, we examine the polarization vectors for values of

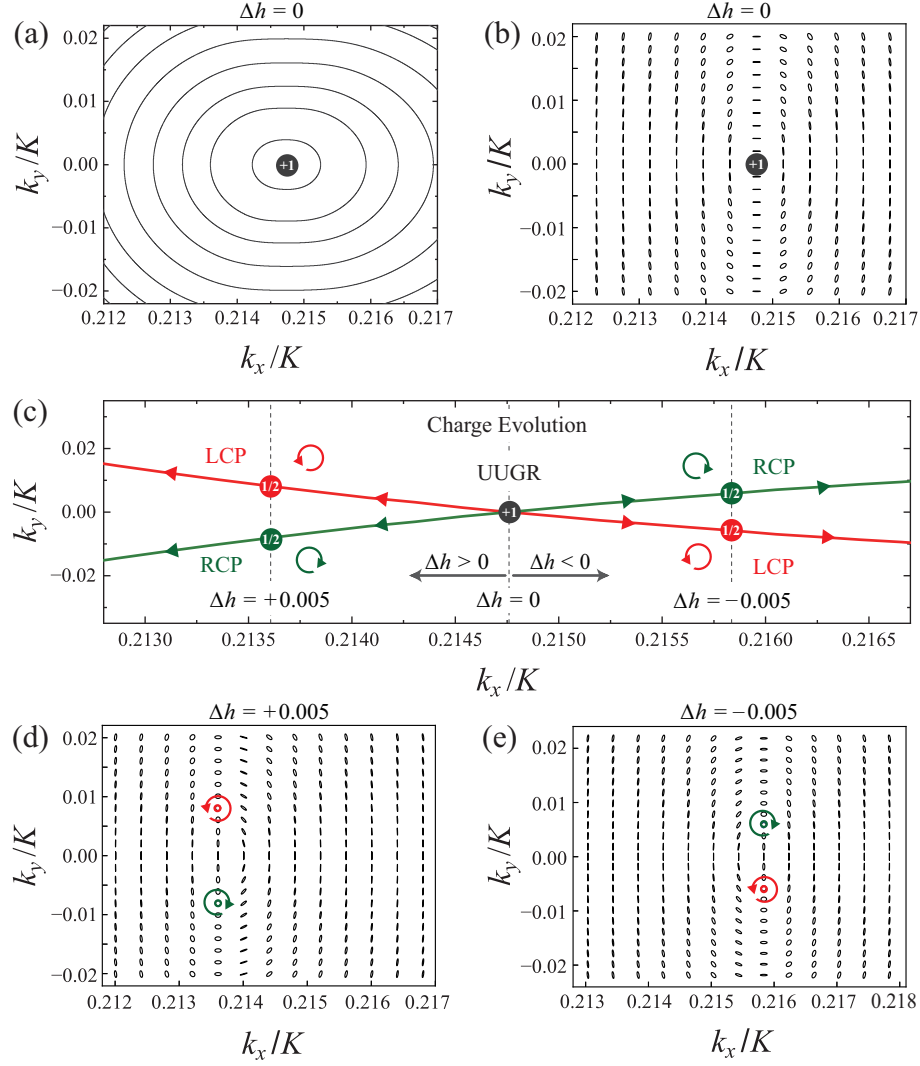

FIG. S2. (a) Polarization vector fields and (b) polarization states of downward radiation at  $h/\Lambda = h_u = 0.2708$ . (c) Illustration of the trajectories traced by paired half-integer topological charges in momentum space as  $\Delta h$  varies. (d) Far-field polarization states observed at  $\Delta h = +0.005$ , and (e) at  $\Delta h = -0.005$ .

$h/\Lambda$  that deviate from  $h_u$ . We define this deviation as  $\Delta h = h/\Lambda - h_u$ . Considering that topological charge is a conserved quantity, when  $|\Delta h| > 0$ , a topological charge of  $q = +1$  splits into two half-integer charges. Figure S2(c) depicts the trajectories of paired  $C$  points, each carrying a topological charge of  $q = +1/2$ , as  $|\Delta h|$  increases from zero. Due to the in-plane mirror symmetry in the  $y$ -direction inherent to the ZCGs, these paired  $C$  points exhibit opposite helicities. Specifically, when  $\Delta h > 0$ , left-handed circularly polarized (LCP) states manifest in the region where  $y > 0$ , while right-handed circularly polarized (RCP)

states appear in the region where  $y < 0$ . Conversely, when  $\Delta h < 0$ , LCP states are observed in the region where  $y < 0$ , and RCP states occur in the region where  $y > 0$ . In this study, the precise locations and helicities of the  $C$  points (or topological charges with  $q = +1/2$ ) are determined by examining the Stokes parameter  $S_3$ .

We next demonstrate the topological nature of the DUGR at  $h/\Lambda = h_d = 0.375$ . The calculated polarization vector fields for upward radiation, as depicted in Fig. S2(a), reveal that the polarization vectors encircle the DUGR positioned at  $(k_x, k_y)/K = (0.213862, 0)$ . The far-field polarization states, as illustrated in Fig. S3(b), reveal that no  $C$  point is observed at  $h/\Lambda = h_d$ . With a deviation  $\Delta h = h/\Lambda - h_d$  different from zero, paired  $C$  points, each carrying half-integer topological charges, emerge from the original topological charge of  $q = +1$ . Figure S3(c) illustrates the trajectories of these paired  $C$  points, which possess opposite helicities, as  $\Delta h$  changes. When  $\Delta h > 0$ , RCP states manifest in the region where  $y > 0$ , while LCP states appear in the region where  $y < 0$ . Conversely, when  $\Delta h < 0$ , RCP states are observed in the region where  $y < 0$ , and LCP states occur in the region where  $y > 0$ . Based on the observations from Fig. S3, it is reasonable to conclude that in ZCGs, the DUGRs induced by interband coupling are situated at the merging points of paired  $C$  points.

- 
- [S1] X. Yin, J. Jin, M. Soljačić, C. Peng, and B. Zhen, “Observation of topologically enabled unidirectional guided resonances,” *Nature* **580**, 467–471(2020).
  - [S2] Y. Zeng, G. Hu, K. Liu, Z. Tang, and C.-W. Qiu, “Dynamics of Topological Polarization Singularity in Momentum Space,” *Phys. Rev. Lett.* **127**, 176101 (2021).
  - [S3] B. Zhen, C. W. Hsu, L. Lu, A. D. Stone, and M. Soljačić, “Topological nature of optical bound states in the continuum” *Phys. Rev. Lett.* **113**(25), 257401 (2014).
  - [S4] T. Yoda and M. Notomi, “Generation and annihilation of topologically protected bound states in the continuum and circularly polarized states by symmetry breaking,” *Phys. Rev. Lett.* **125**, 053902 (2020).
  - [S5] M. Kang, L. Mao, S. Zhang, M. Xiao, H. Xu, and C. T. Chan, “Merging bound states in the continuum by harnessing higher-order topological charges,” *Light Sci. Appl.* **11**, 228 (2022).

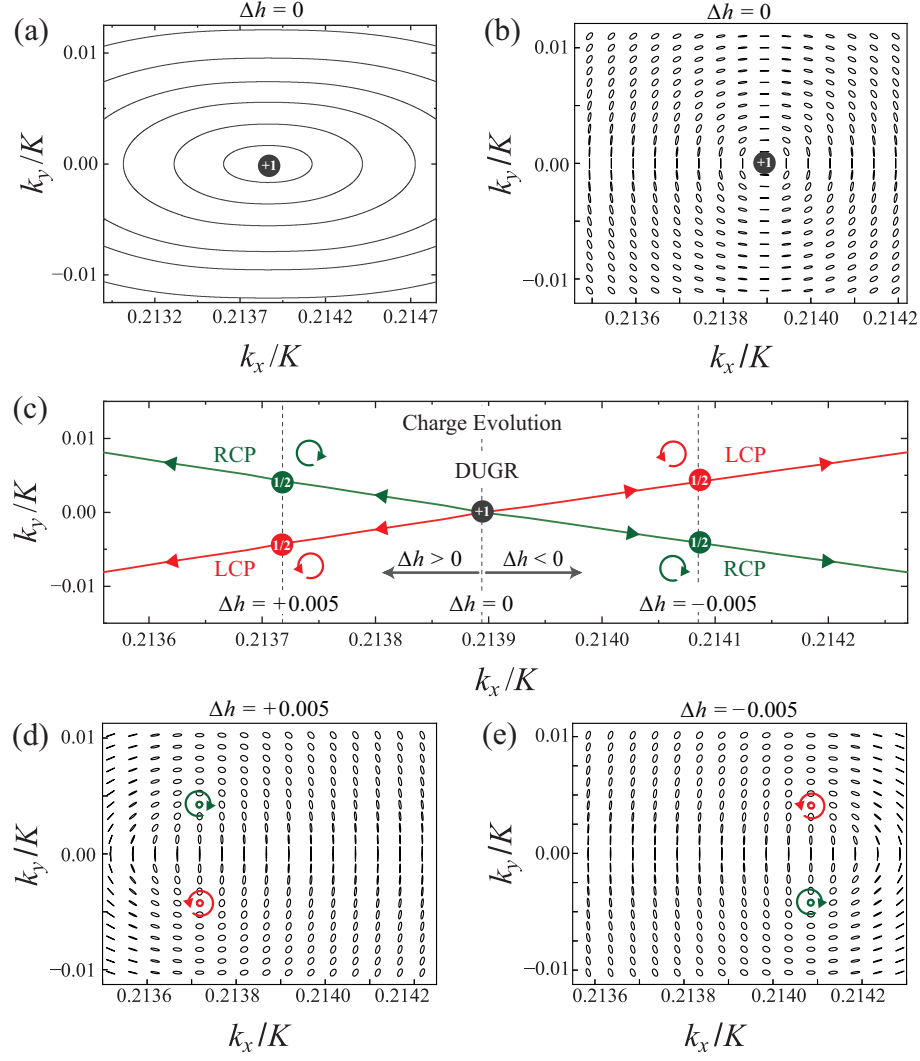

FIG. S3. (a) Polarization vector fields and (b) polarization states of downward radiation at  $h/\Lambda = h_d = 0.379$ . (c) Illustration of the trajectories traced by paired half-integer topological charges in momentum space as  $\Delta h$  varies. (d) Far-field polarization states observed at  $\Delta h = +0.005$ , and (e) at  $\Delta h = -0.005$ .
